# Supplementary material for: A Numerical Approach to Virasoro Blocks and the Information Paradox
Source: arXiv:1703.09727 ancillary file (2017-03-28)

Supplemental Material for:

# A Numerical Approach to Virasoro Blocks and the Information Paradox

by Hongbin Chen, Charles Hussong, Jared Kaplan, and Daliang Li

This Mathematica notebooks contains the implementation of the Zamolochikov's q recursion relation for the Virasoro blocks in 2D CFTs. See the paper for references and further explanation. This code can calculate the first 200 coefficients of the q-expansion in less than 10s, and for 1000 terms in about 45 mins.

*Tested in Mathematica version 11 for Mac OS X.*

For the implementation of this algorithm using C++, please go to `https://github.com/chussong/virasoro`. The C++ code is somehow faster than this Mathematica code, and the q-expansion coefficients used in the paper were obtained using the C++ code.

```
Date[][[1 ;; 3]]
{2017, 3, 28}
```

## Recursion relation of Heavy-light Virasoro blocks

```
ClearAll["Global`*"]


Nprecision = 300;(*Set precision*)
$MinPrecision = Nprecision;

(*qCoeffient returns the q-expansion coefficients. The inputs
  of qCoefficient[] are the the central charge cCentralCharge,
light-operator dimension hLight, the heavy-operator dimension hHeavy,
the intermediate operator dimension hIntermediate,
and the highest power of the coefficients NN wanted.*)

qCoeffient[cCentralCharge_, hLight_, hHeavy_, hIntermediate_, NN_] :=
 Block[{c, hL, hH, b, h, countmn, lengthmn, startmn, Cij, CHij, λLsquare,
   λHsquare, λpq, Ppq, Rmn, RmnDenominator, RmnList, hmnList, mnhalfList,
   temp, NNhalf = Floor[NN / 2], qCoefList = Table[0, Floor[NN / 2] + 1]},

  (*NNhalf is number of terms in the list of the coefficients qCoefList that
   need to be calculated, since only even powers of q are non-zero.*)
```

```
(*Convert the arguments to high
 precision decimals. Do nothing for symbolic calculation.*)
hL = If[NumberQ[hLight], N[Rationalize[hLight], Nprecision], hLight];
hH = If[NumberQ[hHeavy], N[Rationalize[hHeavy], Nprecision], hHeavy];
c = If[NumberQ[cCentralCharge],
   N[Rationalize[cCentralCharge], Nprecision], cCentralCharge];
b = If[NumberQ[c], N[Rationalize[Sqrt[c - 13 + Sqrt[c^2 - 26 c + 25]]/(2 Sqrt[3])], Nprecision], b];
(*For symbolic calculation, present the result in terms of b.*)
h = If[NumberQ[hIntermediate],
   N[Rationalize[hIntermediate], Nprecision], hIntermediate];

λLsquare = 1/4 (b + 1/b)^2 - hL; (*λL^2*)
λHsquare = 1/4 (b + 1/b)^2 - hH; (*λH^2*)
λpq[p_, q_] := 1/2 (p/b + q b); (*λp,q*)

Ppq[p_, q_] := (λpq[p, q]^2 - 4 λLsquare) (λpq[p, q]^2 - 4 λHsquare ) λpq[p, q]^4;
(*Ppq[p,q] gives the contribution to the numerator of Rm,n from λp,q and λ-p,-q*)

RmnDenominator[m_, n_] :=
 Product[Piecewise[{{1, k == 0 && l == 0}, {1, k == m && l == n}}, (k / b + l b) / 2],
  {k, -m + 1, m}, {l, -n + 1, n}];
(*RmnDenominator[m,n] give the denominator of Rm,n,
but only to be used for calculation of the first several terms of Rm,n.*)

(*Rm,n is filled recursively from higher order terms,
but we need to set the boundary values for this recursive calculation.*)
Rmn = Table[0, NN, NN];
Rmn[[1, 2]] = 2 Ppq[0, 1] / RmnDenominator[1, 2];
Rmn[[2, 1]] = 2 Ppq[1, 0] / RmnDenominator[2, 1];
Rmn[[2, 2]] = 2 Ppq[1, -1] Ppq[1, 1] / RmnDenominator[2, 2];
(*Obtain Rm,1 and Rm,2 from Rm-2,1 and Rm-2,2 respectively*)
Do[Rmn[[m, 1]] = Rmn[[m - 2, 1]] / λpq[m - 2, 1] Ppq[m - 1, 0] λpq[m, 1]
    Product[2 / (k / b + nn b), {nn, 0, 1}, {k, {-m + 1, -m + 2, m - 1, m}}], {m, 4, NN, 2}];
```

```
Do[Rmn[[m, 2]] = Rmn[[m - 2, 2]]/λpq[m - 2, 2] Ppq[m - 1, -1] Ppq[m - 1, 1] λpq[m, 2]
   Product[2/(k/b + nn b), {nn, -1, 2}, {k, {-m + 1, -m + 2, m - 1, m}}], {m, 3, NN}];
(*Obtain R_{m,n} from R_{m,n-2}, only calculate terms with even mn*)
Do[Rmn[[m, n]] = If[OddQ[m n], 0, Rmn[[m, n - 2]]/λpq[m, n - 2] λpq[m, n]
    Product[Ppq[p, n - 1], {p, -m + 1, m - 1, 2}] Product[2/(k/b + nn b),
     {nn, {-n + 1, -n + 2, n - 1, n}}, {k, -m + 1, m}]], {m, 1, NN}, {n, 3, NN/m}];

(*In the following calculation,
R_{m,n} and h_{m,n} are stored into one-dimensional tables,
and we only need to consider cases that mn is even*)

startmn = Table[0, Floor[NN/2] + 1];
lengthmn = 0;
Do[startmn[[i]] = lengthmn;
 lengthmn += Length[Divisors[2 i]], {i, 1, NNhalf + 1}];
lengthmn -= Length[Divisors[2 (NNhalf + 1)]];
(*lengthmn counts the length of these one-dimension tables,
which is the sum of the number of divisors of even integers up to NN*)
(*Elements from startmn[[i]]+1 to startmn[[i+1]] of these one-dimensioanl
   tables to be defiend below  correspond to the R_{m,n} and h_{m,n} who have mn/2=i.*)

RmnList = Table[0, lengthmn];
hmnList = Table[0, lengthmn];
mnhalfList = Table[0, lengthmn];

(*RmnList and hmnList are used to stores h_{m,n} and R_{m,n} into a one-
 dimensional tables. Those h_{m,n}s with the same product mn will be stored in
  hmnList from startmn[[mn/2]]+1 to startmn[[mn/2+1]], and similar for RmnList.*)
(*mnhalfList stores the number mn/2 that corresponds to the each element
  in these one-dimensional tables, for example mnhalfList[[1]]=1 (1*2/2==1),
mnhalfList[[2]]=1 (2*1/2==1), mnhalfList[[3]]=2 (1*4/2==2), and so on*)

(*Below is how we construct these one-dimensional tables.*)
countmn = Table[0, NNhalf];
Do[If[EvenQ[m n], (temp = m n/2;
   countmn[[temp]] ++;
   mnhalfList[[startmn[[temp]] + countmn[[temp]]]] = temp;
   RmnList[[startmn[[temp]] + countmn[[temp]]]] = Rmn[[m, n]];
```

```
    hmnList[[startmn[[temp]] + countmn[[temp]]]] = 1/4 (b + 1/b)^2 - λpq[m, n]^2), 0],
  {m, 1, NN}, {n, 1, NN / m}];
 (*countmn[[temp]] records the number of divisors of 2temp that we
  encounters so far, so startmn[[temp]]+countmn[[temp]] is the position
   where the current element should be in these one-dimensional tables*)

 HH = Table[Table[0, startmn[[i + 1]]], {i, 1, NNhalf}];
 (*HH[[i,j]] stores H_{m,n}^k in the diagonal way, as explained in the paper,
 where the fist index corresponds to the total power of H_{m,n}^k, which is i==
  (k+mn)/2 and the second index corresponds to (m,n). The length of HH[[i]] is
   startmn[[i+1]], which is the number of ways to write 2i as 2i==k+mn.*)

 Do[HH[[i, j]] = 1, {i, 1, NNhalf}, {j, startmn[[i]] + 1, startmn[[i + 1]]}];
 (*H_{m,n}^0=1*)

 Cij = Table[RmnList[[j]] / (hmnList[[i]] + 2 mnhalfList[[i]] - hmnList[[j]]),
   {i, 1, lengthmn}, {j, 1, startmn[[NNhalf - mnhalfList[[i]] + 1]]}];
 (*Store the prefactors C_{ij}=R_{p,q}/(h_{m,n}+mn-h_{p,q}) into a two-dimensional table, where the
  first index corresponds to (m,n) and the second index corresponds to (p,q)*)

 CHij = Table[RmnList[[i]] / (h - hmnList[[i]]), {i, 1, lengthmn}];
 (*CHij is the list of prefactor to get the q-
  expansion coefficients in qCoefList, which are denoted as H^k in the paper*)

 Do[Do[HH[[khalf + mnhalfList[[i]], i]] =
     Take[Cij[[i]], startmn[[khalf + 1]]].HH[[khalf]],
   {i, 1, startmn[[NNhalf - khalf + 1]]}], {khalf, 1, NNhalf}];
 (*Calculate the H_{m,n}^k elements, this is the slow part of the code. The
  order that we conduct this calculation is that we calculate all
  the  H_{m,n}^ks with the same k, which can be obtained from HH[[k/2]],
 and then put them in the right places in HH[[]]. This
  process is explained in the Figure 19 of the paper.*)

 qCoefList[[1]] = 1;
 Do[qCoefList[[i + 1]] = Take[CHij, startmn[[i + 1]]].HH[[i]], {i, 1, NNhalf}];
 (*Construct the q-expansion coefficient H^k.*)
 qCoefList]
```

# Examples

## Example 1: c=30, $h_L = 1$, $h_H = 3$, h=0, N=1000

```
qCoeffient[30, 1, 3, 0, 1000] // N // AbsoluteTiming
```

```
(*qCoeffientPublic[] returns a list of the q-expansion coefficients,
starting from the coefficient of q^0, which is 1, and then that of q^2,
q^4, etc. This list only includes coefficients of even powers q^2n,
since the coefficients of odd powers are zero.*)
```

## Example 2: Analytic coefficients

```
(*The code can also be used to obtain the analytic coefficients of the q-
 expansion (the result is given in terms of b). But one should notice that the
  coefficients for hihger powers of q (like q^10) are pretty complicated.*)
```

```
qCoeffient[c, hL, hH, h, 2] // AbsoluteTiming
```

$$\left\{0.000907,\ \left\{1,\ -\frac{4\left(\frac{1}{4b^2}-4\left(\frac{1}{4}\left(\frac{1}{b}+b\right)^2-h_H\right)\right)\left(\frac{1}{4b^2}-4\left(\frac{1}{4}\left(\frac{1}{b}+b\right)^2-h_L\right)\right)}{b^2\left(-\frac{1}{b}+b\right)\left(\frac{1}{b}+b\right)\left(-\frac{1}{4}\left(\frac{1}{b}+b\right)^2+\frac{1}{4}\left(\frac{2}{b}+b\right)^2+h\right)}-\frac{4b^2\left(\frac{b^2}{4}-4\left(\frac{1}{4}\left(\frac{1}{b}+b\right)^2-h_H\right)\right)\left(\frac{b^2}{4}-4\left(\frac{1}{4}\left(\frac{1}{b}+b\right)^2-h_L\right)\right)}{\left(\frac{1}{b}-b\right)\left(\frac{1}{b}+b\right)\left(-\frac{1}{4}\left(\frac{1}{b}+b\right)^2+\frac{1}{4}\left(\frac{1}{b}+2b\right)^2+h\right)}\right\}\right\}$$

## Example 3: Plot the Heavy-Light Virasoro block

```
VBlock[c_, hL_, hH_, h_, N_] :=
  (16 q)^(h - (c-1)/24) z^((c-1)/24 - 2 hL) (1 - z)^((c-1)/24 - hH - hL) EllipticTheta[3, 0, q]^((c-1)/2 - 8 (hH+hL))
   Table[q^i, {i, 0, N, 2}].qCoeffient[c, hL, hH, h, N] /. q → Exp[-π EllipticK[1 - z]/EllipticK[z]];
```

```
Plot[VBlock[30, 1, 3, 0, 10] // Log, {z, 0, 1}]
```

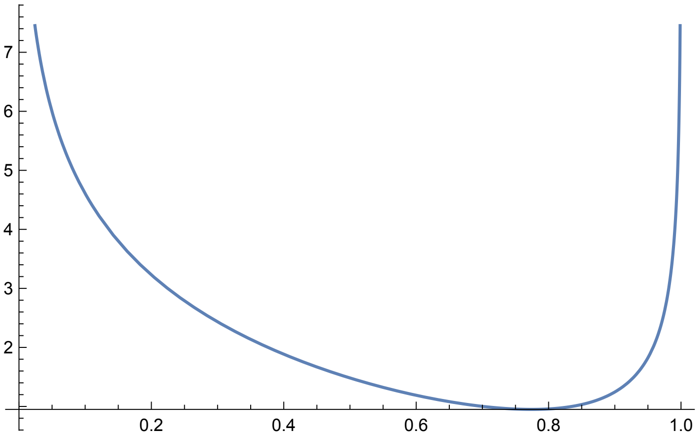


```
(*Series expansion*)
```

```
VBlock[c, hL, hH, 0, 2] /. b -> Sqrt[-13 + c + Sqrt[25 - 26 c + c^2]]/(2 Sqrt[3]) // Series[#, {z, 0, 2}] & //
  Series[#, {c, Infinity, 1}] & // Normal
```

$$z^{-2\,hL}\left(1+\frac{2\,hH\,hL\,z^{2}}{c}\right)$$

## Example 4: Lorentzian time behavior of the Virasoro block

```
(*Analytic continuation to Lorentzian time*)
EK[r_, t_] := EllipticK[1 - r E^(-i t)] - 2 i (1 + Floor[(-t - π)/(2 π)]) EllipticK[r E^(-i t)];
qVal[r_, t_] := Exp[-π EllipticK[r E^(-i t)]/EK[r, t]];

VBlockLorentzian[c_, hL_, hH_, h_, N_, r_] :=
  (16 q)^(h - (c-1)/24) z^((c-1)/24 - 2 hL) (r)^((c-1)/24 - hH - hL) E^(-i t ((c-1)/24 - hH - hL)) EllipticTheta[3, 0, q]^((c-1)/2 - 8 (hH+hL))
    Table[q^i, {i, 0, N, 2}].qCoeffient[c, hL, hH, h, N] /.
   {q -> qVal[r, t], z → 1 - r E^(-i t)};

VBlockLorentzian[30, 1, 3, 0, 200, 0.3] // Abs // Log;
Plot[%, {t, 0, 30}]
```

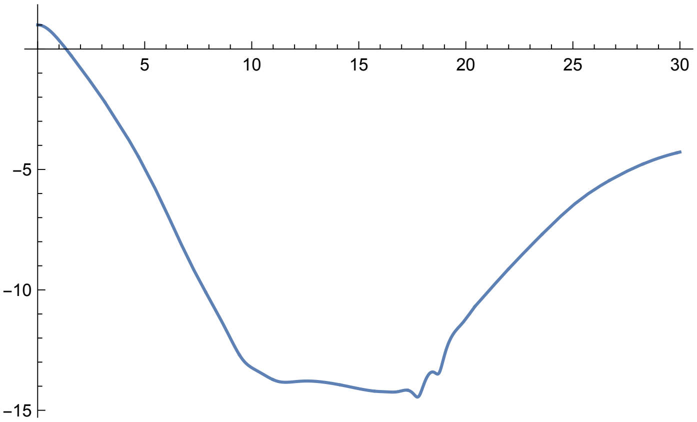

Supplement: Supplementary file 1 [file Virasoro_q_Expansion.pdf]
